# Supplementary material for: Polarization-Tuned Fano Resonances in All-Dielectric Short-Wave Infrared Metasurface
Source: arXiv:2212.00758 ancillary file (2022-12-01)
Supplement: Supplementary file 1 [file Supporting_information.pdf]

# Supplementary information:
# Polarization-Tuned Fano Resonances in All-Dielectric Short-Wave Infrared Metasurface

Anis Attiaoui,[1] Gérard Daligou,[1] Simone Assali,[1] Oliver Skibitzki,[2] Thomas Schroeder,[3] and Oussama Moutanabbir[1]

[1] *Department of Engineering Physics, École Polytechnique de Montréal, C.P. 6079, Succ. Centre-Ville, Montréal, Québec, Canada H3C 3A7*

[2] *Leibniz-Institut für innovative Mikroelektronik, Im Technologiepark 25, 15236 Frankfurt (Oder), Germany*

[3] *Leibniz-Institut für Kristallzüchtung, Max-Born-Straße 2, 12489 Berlin, Germany*

## Contents

Supplementary Note 1. Reflectance Measurements of Si/Ge NW Arrays 2

Supplementary Note 2. Structural characterization of Si/$Ge_{0.9}Sn_{0.1}$ core/shell array 3

Supplementary Note 3. Transmission of the Si/GeSn NW array 5

Supplementary Note 4. Absorption Measurement of Si/$Ge_{0.9}Sn_{0.1}$ NW array 6

Supplementary Note 5. Lineshape Model Fit 7

Supplementary Note 6. All-Dielectric Refractive Index Sensing Literature Review 8

Supplementary Note 7. 3D FDTD Simulation of Core/Shell NWs 9

- S7.1 Multipolar Decomposition 9
- S7.2 Coupled Harmonic Oscillator Model Fit 9
- S7.3 Effect of Shell Diamater on the Fano Resonance 11
- S7.4 Effect of Periodicity on the Fano Resonance Features 12

Supplementary Note 8. Structural Characterization of the Reference $Ge_{0.9}Sn_{0.1}$ layer on Ge-VS/Si 13

Supplementary Note 9. Geometrical Parameters of the Core/Shell NW Array 14

References 15

**Supplementary Note 1. Reflectance Measurements of Si/Ge NW Arrays**

To better understand the effect of the GeSn shell on reflectance, three different Si/Ge nanowire (NW) arrays were grown with variable Ge shell thickness of 45 nm, 120 nm, and 200 nm, as shown in the scanning electron microscope (SEM) micrographs in Fig. S1b. The unpolarized specular reflectance ($R$) (average of the $s$- and $p$-polarized $R$), at near-normal angle of incidence (AOI) of 6°, is compared for all the fabricated nanostructures, as shown in Fig. S1a. Clearly, the reflectance is reduced from 48% for Si bulk to less than 10% for the Si/GeSn array. On the one hand,

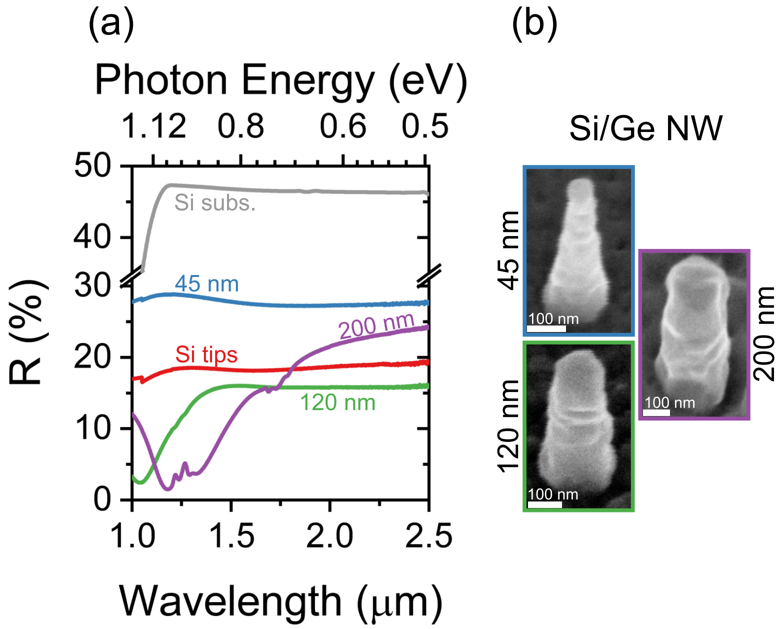


Figure S1. (a) Unpolarized specular reflectance of Si substrate and different nanostructures. The reflectance of Si nanotips is shown. The reflectance spectra of variable shell thickness of Si/Ge core/shell NW is also presented. The shell thickness is increased from 45 nm to 200 nm, as shown in the SEM images of panel (b).

increasing the Ge shell-in average- from 45 nm to 200 nm decreases light reflectance and increases the shell surface roughness due to preferential Ge sidewall diffusion. The Si array reflectance (red line in Fig. S1a) is almost independent of the photon energy with an average of approximately 18.5 %, which is 11.5% smaller than that of the Si bulk (gray line in Fig. S1a). The reflectance is reduced with respect to that of the bare substrate. This reduction results from the lower index of refraction in the array, making it a stepped-index antireflection coating. [1] This agrees qualitatively well with previous measurement of straight Si NWs of 45±10 nm diameter and 1 μm height. [2] On the other hand, with 45 nm Ge shell, the Si/Ge array (blue line in Fig. S1a) behave similarly to the Si tips, meaning that the shell is too thin to contribute to an efficient light absorption. Increasing the shell to 120 nm (green line in Fig. S1a) reduces the reflectance below the Si tips with a remarkable decrease around 1 μm (below 3%) associated with a clear cut-off (around 1.45 μm) emanating from the Ge shell direct band gap (near 0.8 eV ∼ 1.55 μm). Finally, at a Ge shell thickness of 200 nm (purple line in Fig. S1a), the reflectance minimum is redshifted with the appearance of new surface-related diffraction modes near 1.4 μm and resonant features near 1.7 μm, that are absent for the 45 nm and 120 nm Si/Ge arrays. This emphasizes the shell-dependent origin of the aforementioned observed features.

Finally, to study the low reflectance of the core/shell array in more depth for a wide range of AOI, the angle-resolved specular reflectance ratio $\eta_R$ between 6° to 52° was measured for both s- and p-polarizations, as shown in Fig. S2a-b. Briefly, a p-polarized incident light coincides with a $\varphi = 0°$, that is, polarization along the x-direction, whereas an s-polarized state corresponds to a $\varphi$ of 90° (along the y-direction). The measured specular reflectance of the array is lower than that of the Si array in the wavelength range between 1 μm and 2.2 μm.

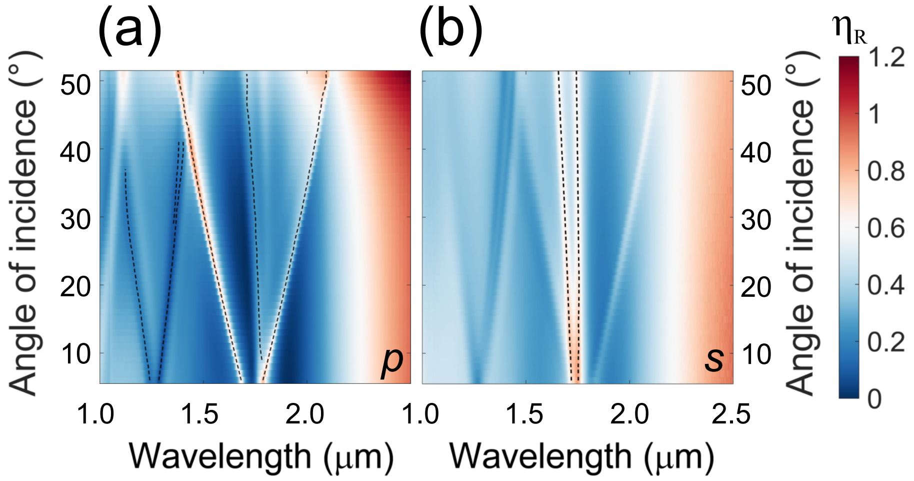


Figure S2. (a-b) Polarization-dependant dispersion maps of the Si/GeSn NW array measured at (a) *p*- and (b) *s*-polarization. The dashed lines are a guide to eye to follow the main resonant features.

### Supplementary Note 2. Structural characterization of Si/$Ge_{0.9}Sn_{0.1}$ core/shell array

To elucidate the structural properties of the Si/$Ge_{0.9}Sn_{0.1}$ core/shell NWs, cross-sectional transmission electron microscopy (TEM) measurements are performed. The scanning-TEM (STEM) and associated electron energy loss spectroscopy (EELS) images of the Si, Ge, and Sn elements are displayed in Fig. S3a. The $Ge_{0.9}Sn_{0.1}$ shell with a thickness of 100-150 nm is visible through the whole length of NW, without being significantly affected by the change in the Si core diameter. By counting the missing wires in a low magnification SEM image (not-shown here), the defect rate of the array can be estimated to be as low as 3.5%, confirming the high conformal growth yield.

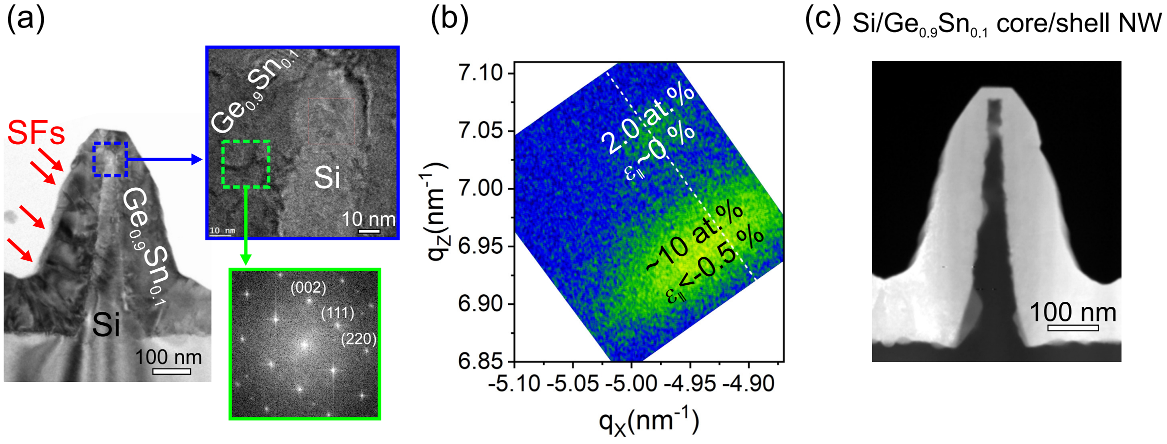


Figure S3. (a) High-resolution TEM (HRTEM) images acquired at multiple locations of the Si-GeSn interface and corresponding Fast-Fourier transform (FFT) images are shown. Local crystalline pockets of SiGe intermixing are observed near the interface. (b) RSM map around the asymmetrical (224) reflection plane of the metasurface. A $\sim$ 10 at.% Sn peak with a residual compressive strain ($\varepsilon_{\|}$) $< -0.5\%$ is visible, with a very broad nature indicating a reduced crystal quality of the GeSn as a result of the plastic relaxation. (c) HRTEM map of a single Si/$Ge_{0.9}Sn_{0.1}$ NW.

High-resolution transmission electron microscopy (HRTEM) images acquired at multiple locations of the Si-GeSn interface and corresponding Fast-Fourier transform (FFT) images are shown in Fig. S3a. Epitaxial relation between the Si core and the GeSn shell is observed through the whole interface even when local pockets of SiGe intermixing are present. These SiGe pockets inside the Si NW core are single crystalline and could originate from enhanced diffusion of the atomic species during the initial stages of the coherent growth [3] of the GeSn shell. However, as the shell grows

thicker, the critical thickness for strain relaxation $h_C$ is quickly reached ($h_C << 10\,\mathrm{nm}$) and multiple stacking faults (SFs) nucleate in the GeSn shell. These defects originate at the interface with the Si core and then propagate through the thickness of the shell. To investigate the structural properties of the NWs at a larger scale, X-ray diffraction (XRD) measurements are performed. To decouple strain and composition in GeSn, reciprocal space mapping (RSM) around the asymmetrical (224) XRD peak is performed as shown in Fig. S3b. A ∼10 at.% Sn peak with a residual compressive strain $\varepsilon_{\parallel} < -0.5\%$ is visible. However its very broad nature indicates a reduced lower crystal quality of the GeSn as a result of the plastic relaxation indeed observed in the TEM images in Fig. S3a. In addition, a low intensity ∼2 at.% Sn peak ($\varepsilon_{\parallel} \sim 0\%$) is present in the RSM measurement. A ∼1 at.% Sn peak, at the equilibrium solubility of Sn in Ge, is commonly observed in GeSn where phase separation and segregation of Sn at the surface take place during growth or post-growth thermal treatments [4]. However, the ∼2 at.% peak seems to exclude the presence of Sn segregation in the NWs, in agreement with the absence of Sn droplets on the NW sidewall [5] in the scanning transmission electron microscopy (STEM) images in Fig. S3a. Thus, an intermediate $Ge_{0.98}Sn_{0.02}$ layer most likely develops in the early stages of the shell growth, hence in the proximity with the interface with the Si core.

The highly conformal GeSn growth extends all the way to the Si substrate and to the neighboring NWs, without the formation of macroscopic Sn droplets. This is a clear indication that Sn segregation and phase separation in GeSn are strongly minimized, if not suppressed. Interestingly, multiple SiGe intermixing spots (Ge∼30-40 at.% compositional range) are present across the length of the Si NW core and on the surface of the Si wafer. No correlation between the Si-Ge intermixing and Si NW diameter clearly emerges from the data, and it remains visible even at the smallest Si NW diameters. This observation suggests that strain remains high enough to promote Ge diffusion in the Si NWs, even when the core diameter decreases to $\sim 20\,\mathrm{nm}$. In addition, SiGe pockets with smaller size are also visible at the interface with the Si substrate, thus indicating the intermixing is not limited to the NW region only. No significant diffusion of Si into GeSn is observed. Moreover, because of the extremely low equilibrium solubility of Sn in Si (<0.1 at.%), [6] diffusion of Sn into Si NWs is also suppressed. Thus, the high tensile strain (>5 %) induced on the Si NWs/substrate by the $Ge_{0.9}Sn_{0.1}$ shell growth seems to activate SiGe intermixing at a very low growth temperature of 300°C. We note that strain partitioning between the Si core and the GeSn shell is expected to reduce strain in the growing shell [7, 8] and contribute to preserve the metastable state of the GeSn alloy.

**Supplementary Note 3. Transmission of the Si/GeSn NW array**

The metasurface was grown on a single-side polished Si substrate. This has inhibited any spectral transmission ($T$) measurements. To that end, finite-difference time domain (FDTD) simulation were undertaken to quantify the transmittance of the metasurface and evaluate the modulation depth defined as $|(T_{\text{on}} - T_{\text{off}})/T_{\text{on}}| \times 100\%$, where $T_{\text{on}}$ and $T_{\text{off}}$ represent the transmittance with the maximized polarization-induced resonance (PIR) (at $\varphi = 0°$) and without PIR effect (at $\varphi = 90°$), respectively. Fig. S4 shows the transmittance spectra of the Si/GeSn metasurface at AOI of 6°.

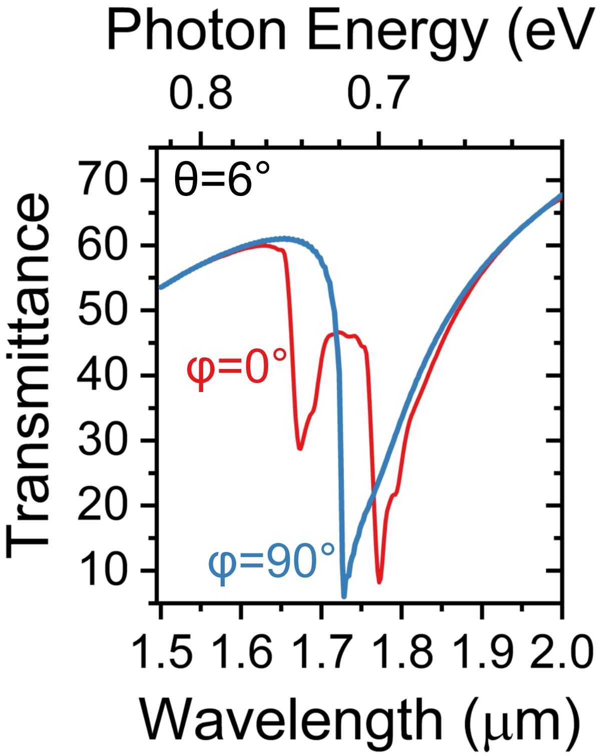


Figure S4. Simulated transmittance of the Si/GeSn core/shell NW array at an angle of incidence of 6° and two different polarization $\varphi = 0°$ and 90°. The PIR is very clear with a modulation depth of 75%.

### Supplementary Note 4. Absorption Measurement of Si/$Ge_{0.9}Sn_{0.1}$ NW array

Using an integrating sphere equipped with an InGaAs detector, the diffuse, specular, total reflectance, and absorptance of the Si/GeSn NW array were measured as shown in Fig. S5. The Fano resonances are only present in the reflectance measurement confirming that the observed behavior is modulated by the metasurface itself.

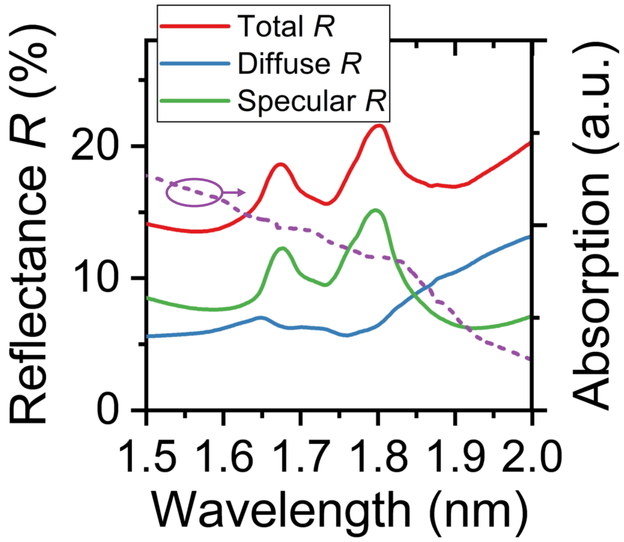


Figure S5. (a) Unpolarized specular reflectance of Si substrate and different nanostructures. The reflectance of Si nanotips is shown. The reflectance spectra of variable shell thickness of Si/Ge core/shell NW is also presented. The shell thickness is increased from 45 nm to 200 nm, as shown in the SEM images of panel (b).

## Supplementary Note 5. Lineshape Model Fit

TABLE S1. Extracted fitting parameters from the lineshape model (Eq. **??**) for variable polarization angle $\varphi$.

| polarization ($\varphi$) | $\omega_1$ **(nm)** | $\gamma_1$ **(nm)** | $\omega_2$ **(nm)** | $\gamma_2$ **(nm)** | **b** | **q** |
|---|---|---|---|---|---|---|
| 0 | 1684.6 | 17.12 | 1785.0 | 23.54 | 1.29 | -1.28 |
| 10 | 1683.9 | 17.36 | 1784.7 | 24.18 | 1.42 | -1.24 |
| 20 | 1682.9 | 18.89 | 1784.1 | 26.50 | 1.69 | -1.08 |
| 30 | 1685.7 | 24.97 | 1780.9 | 31.58 | 1.83 | -0.82 |
| 40 | 1688.4 | 22.00 | 1754.9 | 45.40 | 1.03 | -0.25 |
| 50 | 1684.5 | 10.51 | 1736.8 | 45.16 | 0.70 | 0.00 |
| 60 | 1680.2 | 33.93 | 1733.5 | 36.20 | 0.15 | -0.10 |
| 70 | 1742.0 | 34.82 | | 29.87 | 3.30 | 0.00 |
| 80 | 1745.0 | 32.80 | | 28.60 | 3.47 | -0.30 |
| 90 | 1747.4 | 32.48 | | 29.10 | 3.19 | -0.55 |

## Supplementary Note 6. All-Dielectric Refractive Index Sensing Literature Review

TABLE S2. Comparison of the performance of various experimentally-designed all-dielectric based RI sensors with the corresponding geometry, the material used, the accessible spectral range, the $Q$-factor, and RI sensitivity $S$.

| Geometry | Material | Spectral range | $Q$-factor | Sensitivity $S$ | Reference |
|---|---|---|---|---|---|
| Rectangular bar and ring resonators array | Si | $1.32 - 1.42\,\mu m$ | $\sim 30000$ | 289 nm/RIU | [9] |
| Two-asymmetric split ring resonators | Si<br>PDMS | $0.6 - 1.1\,THz$ | $\sim 75.7$ | 231 GHz/RIU | [10] |
| Subwavelength grating microring resonator | Si | $1.525 - 1.565\,\mu m$ | $\sim 9100$ | 440.5 nm/RIU | [11] |
| Photonic crystal | SOI | $1.534 - 1.542\,\mu m$ | $\sim 2828$ | 303 nm/RIU | [12] |
| Single NW | CdSe/ZnS QDs doped PLA† NW | $0.4 - 1\,\mu m$ | $\sim 4$ | 834 nm/RIU | [13] |
| Core/shell NW arrays | $Si/Ge_{0.9}Sn_{0.1}$ | $1.6 - 2.0\,\mu m$ | $\sim 57/40$ ‡<br>$\sim 30.5$ ⋆ | 81/149 nm/RIU<br>386 nm/RIU | **This work** |

† polylactic acid
‡ from ED/MD modes at $\varphi = 0°$
⋆ from Fano resonance at $\varphi = 90°$

## Supplementary Note 7. 3D FDTD Simulation of Core/Shell NWs

### S7.1. Multipolar Decomposition

FDTD simulations are performed based on the commercial software Ansys-Lumerical© to investigate the scattering of a plane wave incident on the single $Si/Ge_{0.9}Sn_{0.1}$ NW. As presented in Fig. S6a, a plane wave is injected along the

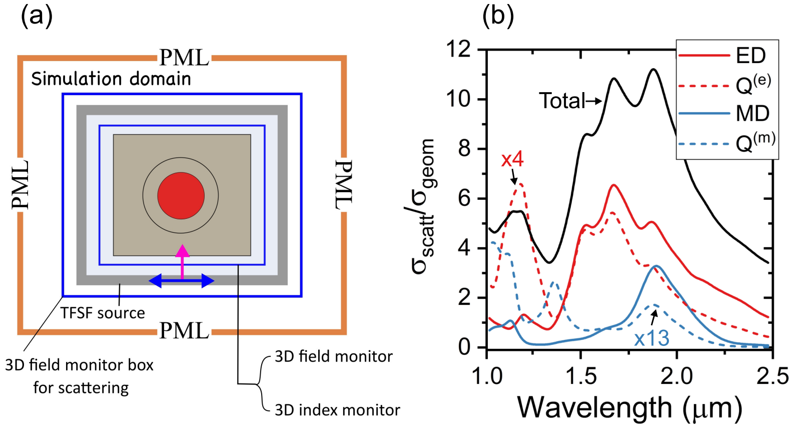


Figure S6. (a) Schematic illustration of the top view of the FDTD simulation domain. (b) Calculated scattering cross sections from each multipole contribution (ED, MD, $Q^{(e)}$, and $Q^{(m)}$) and the total sum of them at $\varphi = 0°$.

$y$-axis into the simulation domain, using a total-field/scattered-field (TFSF) source. Unlike the usual plane wave source, this source separates the scattered field from the incident field, making the scattering analysis straightforward. The 3D field and index monitors inside the TFSF box are used to record the electric field and the refractive indexes of the structure, respectively. A field monitor is added outside the TFSF source box to record the total scattering cross-section. Moreover, Perfectly matched layer (PML) boundary conditions are used in both horizontal and vertical directions to prevent unphysical scattering and reflection at the edge of the simulation box. Different simulations were performed with the polarization angle $\varphi$ of the incident wave changing from 0° to 90°. Besides, a multipolar decomposition is performed using the theoretical method developed by Alaee *et al.* [14] and the MATLAB© implementation by Hinamoto *et al.* [15]. This process is mainly used to investigate the impact of the polarization on the multipole moments and their contributions to the total scattering cross-sections. These moments, computed using the electric field and the refractive index extracted during the FDTD simulations, are used to evaluate the contribution of each of the different scattering cross-sections (Fig. S6b).

### S7.2. Coupled Harmonic Oscillator Model Fit

The coupled differential equations, represented by Eq. 4 in the main text, can be solved numerically with Matlab following the matrix approach. However, for our situation, only the displacement $x_1$ of the first oscillator was required to simulate the reflectance spectra at each polarization angle $\varphi$. By assuming the displacements of the oscillators to be harmonic, such that $x_1(t,\varphi) = c_1(\varphi)e^{i\omega t}$ and $x_2(t,\varphi) = c_2(\varphi)e^{i\omega t}$, the amplitude of the first oscillator is analytically derived and given by

$$c_1(\varphi) = \frac{\omega_2^2-\omega^2+i\omega\gamma_2}{(\omega_2^2-\omega^2+i\omega\gamma_2)(\omega_1^2-\omega^2+i\omega\gamma_1)-\omega^2\tilde{\kappa}'^2} \times \alpha E_0|\cos\varphi| \tag{S1}$$

The squared modulus of the solution $|c_1(\varphi)|^2$ was used to fit the experimental data for each polarization angle $\varphi$. To accurately describe the features observed in the reflectance spectra, the coupling coefficient $\tilde{\kappa}'$ was considered complex with an amplitude $\tilde{\kappa}$ and a phase $\phi_k$. The amplitude $E_0$ of the electromagnetic field was considered constant and set to one to reduce the number of fitting parameters involved in the model. As a result the fitting parameters were the frequencies $\omega_1, \omega_2$, the damping $\gamma_1, \gamma_2$, the coupling strength $\alpha$, the coupling amplitude $\tilde{\kappa}'$, and the phase $\phi_k$. The full fitting process was achieved using LMFIT, a non linear least-squares minimization python package from Newville *et al*[16]. The fitting curves are shown in Fig. S7, with the extracted fitting parameters given in Table S3.

Moreover, the effect of the coupling strength $\tilde{\kappa}$ on the reflectance ratio $\eta_R$ have been investigated at different polarization angle $\varphi(= 0°, 30°, 60°, 90°)$. While keeping all the other fitting parameters to their values extracted

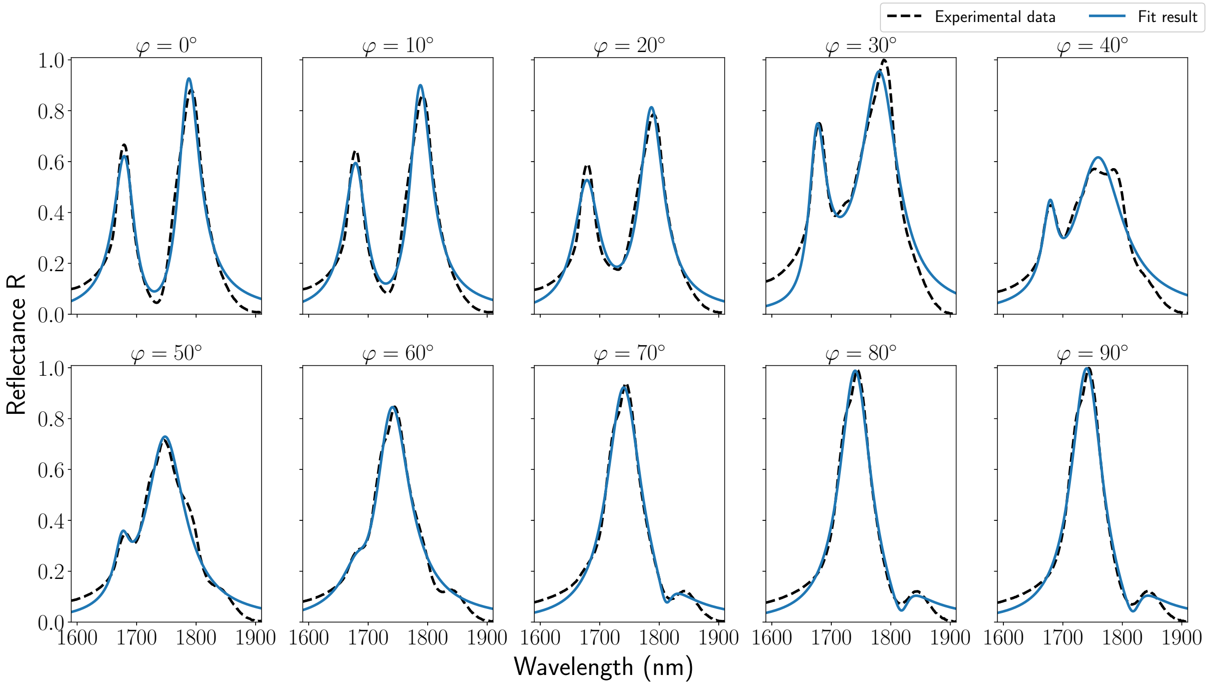


Figure S7. Polarization-dependent reflectance ratio $\eta_R$ characterization at a fixed AOI of 6°. Simulation of the polarization-dependent reflectance spectra. The simulated reflectance spectra are shown as blue trace at each polarization.

TABLE S3. Extracted Parameters from the CHO model for variable polarization

| polarization ($\varphi$) | $\omega_1$ **(nm)** | $\gamma_1$ **(nm)** | $\omega_2$ **(nm)** | $\gamma_2$ **(nm)** | $\tilde{\kappa}$ **(meV)** | $\phi_k$ **(rad)** | $\alpha$ **($\pm 8 \times 10^{-4}$)** |
|---|---|---|---|---|---|---|---|
| 0 | $1736.12 \pm 0.21$ | $30.43 \pm 1.86$ | $1729.27 \pm 0.17$ | $56.04 \pm 1.68$ | $43 \pm 0.27$ | 0 | 0.0458 |
| 10 | $1735.46 \pm 0.2$ | $19.05 \pm 2$ | $1729.27 \pm 0.17$ | $69.99 \pm 1.81$ | $44.6 \pm 0.36$ | 0 | 0.0447 |
| 20 | $1734.37 \pm 0.2$ | $0 \pm 2.59$ | $1728.81 \pm 0.18$ | $99.49 \pm 2.41$ | $48.7 \pm 0.64$ | 0 | 0.0439 |
| 30 | $1776 \pm 2.31$ | $0 \pm 4.22$ | $1680.14 \pm 2.3$ | $104.9 \pm 4.01$ | $51.1 \pm 1.68$ | $5.6602 \pm 0.03$ | 0.0502 |
| 40 | $1752 \pm 1$ | $78.22 \pm 2.4$ | $1684.54 \pm 1.22$ | $45.19 \pm 2.43$ | $23.8 \pm 0.76$ | $5.6211 \pm 0.03$ | 0.0676 |
| 50 | $1742.44 \pm 0.76$ | $64.47 \pm 1.64$ | $1680.32 \pm 1.31$ | $44.97 \pm 2.41$ | $20.2 \pm 0.68$ | $2.5137 \pm 0.03$ | 0.0723 |
| 60 | $1732.11 \pm 0.41$ | $72.84 \pm 0.77$ | $1692.21 \pm 0.83$ | $45.61 \pm 3.05$ | $14.5 \pm 0.62$ | 0 | 0.0973 |
| 70 | $1740.29 \pm 0.43$ | $80.43 \pm 0.97$ | $1812.04 \pm 0.84$ | $17.43 \pm 1.72$ | $15.8 \pm 0.53$ | $2.5523 \pm 0.03$ | 0.1343 |
| 80 | $1743.15 \pm 0.53$ | $81.54 \pm 1.17$ | $1818 \pm 0.81$ | $17.55 \pm 1.86$ | $21.1 \pm 0.59$ | $2.6695 \pm 0.02$ | 0.2628 |
| 90 | $1743.53 \pm 0.55$ | $82.12 \pm 1.21$ | $1818 \pm 0.8$ | $17.55 \pm 1.9$ | $21.9 \pm 0.59$ | $2.68 \pm 0.02$ | 0.0457 |

previously, the coupling parameter $\tilde{\kappa}$ was changed from 0 to 0.15 eV at each polarization angle. The corresponding simulated normalized reflectance spectra are displayed in Fig. S8 for both $s$ and $p$ polarization, as well as $\varphi = 30°$ and 60°. For $\varphi = 0°$ and $\varphi = 60°$, where the coupling coefficient $\tilde{\kappa}'$ is real ($\phi_k = 0$), the typical behavior of the EIT effect—a dip emerging on the broad reflectance feature—is observed. However, for the two remaining polarization, completely different effect have been observed.

Regarding the 30° polarization, an extremely sharp resonance peak ($P_1$) is observed around 1776 nm for $\tilde{\kappa} = 0$. With the increasing values of $\tilde{\kappa}$, this peak is broadened, and a second peak ($P_2$) around 1677 nm starts to be more visible. From $\tilde{\kappa} \sim 50$ meV, $P_1$ loses intensity to $P_2$, until it completely vanishes at $\sim 67$ meV, where $P_2$ shifts to a slightly lower wavelength and becomes extremely sharp. Shortly after this value of $\tilde{\kappa}$, $P_2$ starts to broaden and blue-shift. A similar behavior is also observed at $\varphi = 90°$, where the initially broadened spectrum centered around 1744 nm becomes sharper while shifting to lower wavelengths. This trend is still observed until the coupling strength reaches 62 meV, and an extremely sharp peak is observed. These different results highlight the importance of the coupling coefficient in the a dynamic control of the resonance response.

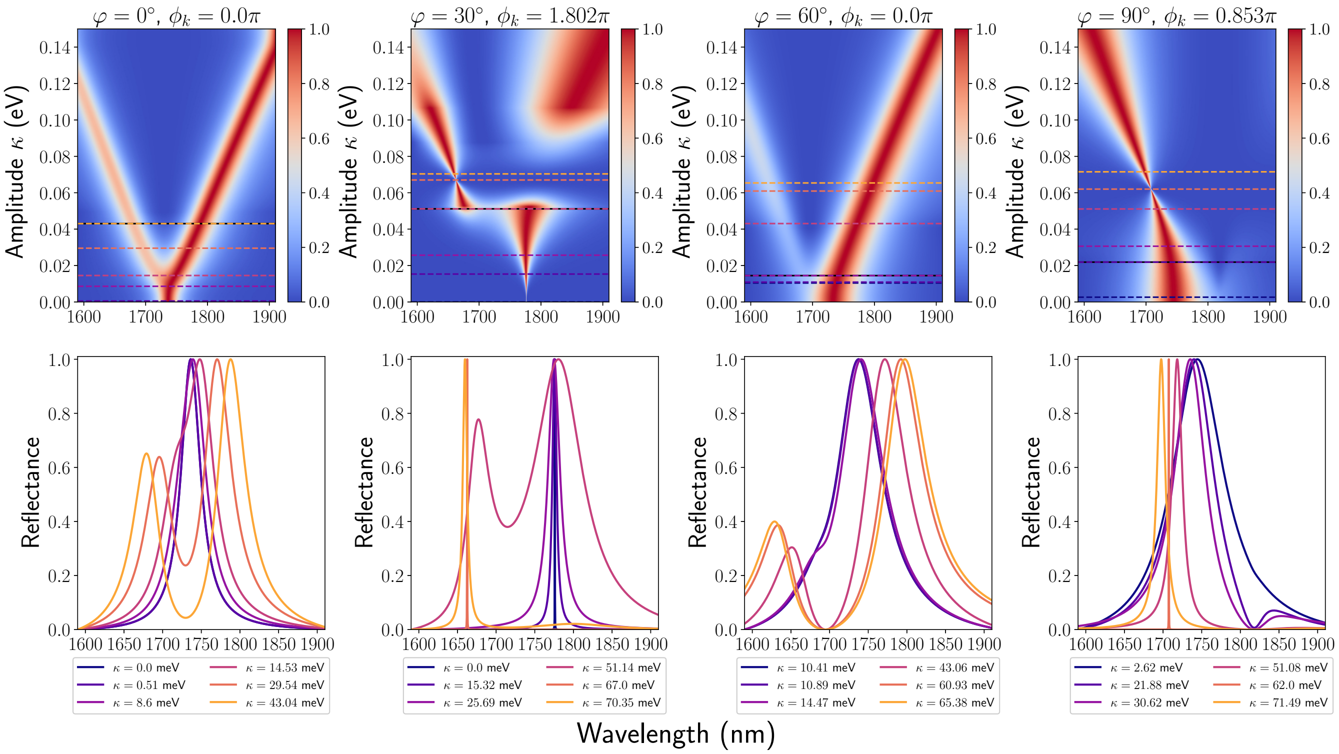


Figure S8. Effect of the coupling strength $\tilde{\kappa}$ on the reflectance ratio $\eta_R$. The polarization-dependent reflectance maps in the first row highlight the effect of $\tilde{\kappa}$ over the resonance peaks. For the second row, specific values of $\tilde{\kappa}$ have been chosen to emphasize some of the interesting features that have been observed on the map.

### S7.3. Effect of Shell Diamater on the Fano Resonance

To highlight the relationship between the geometry of the core/shell NW and the Fano resonance lineshape (Fig. S9a), a simulation of the reflectance was undertaken by changing the bottom shell diameter $d_{sB}$ from 150 nm to 300 nm while keeping the top shell diameter $d_{sT}$ fixed to 80 nm. Noticeably, as $d_{sB}$ increases, the FWHM of the ED and MD modes increases, which translate to a decrease in the asymmetry parameter $|q|$, as shown in Fig. S9b.

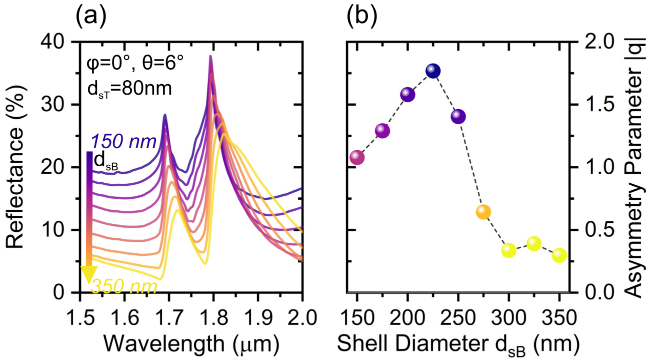


Figure S9. (a) FDTD reflectance spectra of the Si/GeSn core/shell metasurface for a fixed top shell diameter $d_{sT}$ of 80 nm and a variable shell diameter $d_{sB}$ from 150 nm to 300 nm. (b)The color-coded SEM images shows the fabricated arrays for 4 specific periods (500 nm to 2 μm from bottom to top). The gray line is a guide to the eye to follow the Fano resonances. The scale bar in all SEM images is fixed to 1 μm.

### S7.4. Effect of Periodicity on the Fano Resonance Features

To study how the Fano resonance asymmetry is effected by the modification in the near field coupling between the NWs, a combined theoretical and experimental investigation were undertaken. First, the polarization and incident angle were fixed to 0° and 6°, respectively. Second, four different Si/$Ge_{0.9}Sn_{0.1}$ core/shell NW metasurfaces were fabricated with a variable pitch $p$ from 500 nm to 2 µm, as shown in Fig. S10. The corresponding reflectance ratio $\eta_R$ is shown for each metasurface. To better visualize the Fano resonances, we also simulated, using FDTD, $\eta_R$ at variable pitch $u$ between 400 nm and 2 µm. There is a clear redshift in the ED and MD modes, driven by the diffraction effect of the metasurface. Not only that, the lineshape broadening of the MD mode changes from a broad resonance ($u < 450$ nm) to a sharper one ($450\,\text{nm} < u < 525$ nm). When $u > 575$ nm, the Fano resonance effect disappear confirming the interplay between the surface diffraction resonant modes and the dipole resonances.

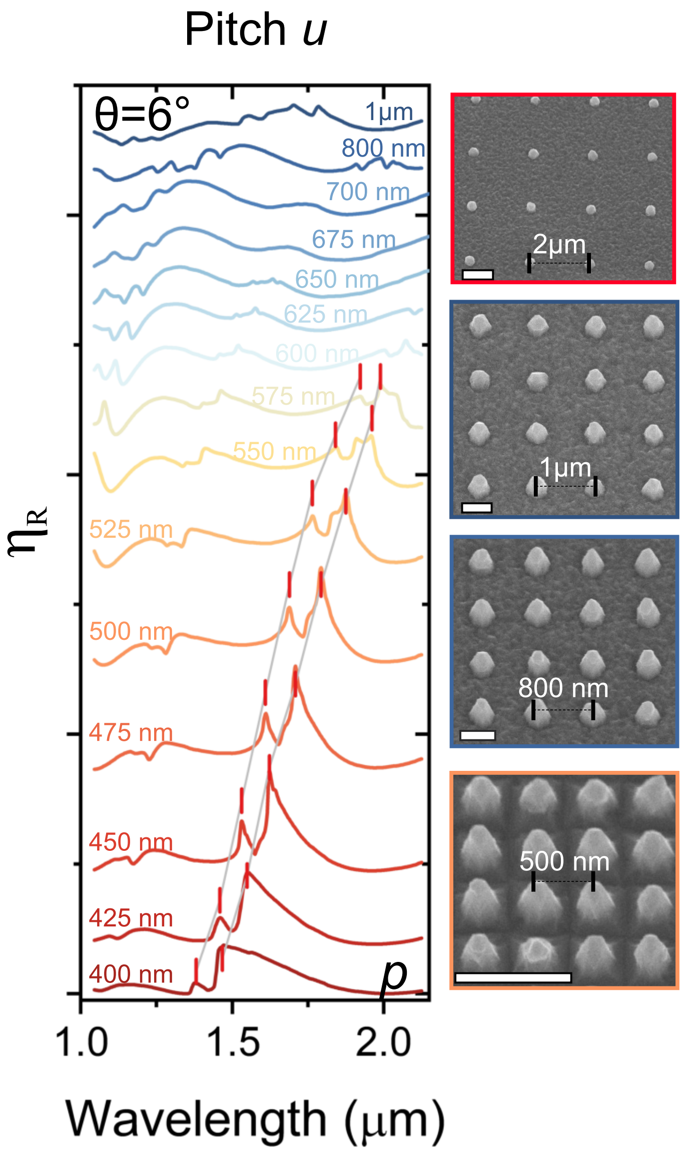


Figure S10. (a-b) The color-coded SEM images shows the fabricated arrays for 4 specific periods (500 nm to 2 µm from bottom to top). The gray line is a guide to the eye to follow the Fano resonances. The scale bar in all SEM images is fixed to 1 µm.

**Supplementary Note 8. Structural Characterization of the Reference $Ge_{0.9}Sn_{0.1}$ layer on Ge-VS/Si**

The reference $Ge_{0.9}Sn_{0.1}$ thin film grown was grown inside a low-pressure chemical vapor deposition (CVD) at 300 °C on top of a Ge-virtual substrate and a 4-inch Si wafer. The cross-sectional TEM image (Fig. S11a) reveals the localisation of defects near the interface between Si/Ge and Ge/$Ge_{0.9}Sn_{0.1}$ interfaces. Additionally, some threading dislocations are also seen. Finally, reciprocal space mapping (RSM) around the asymmetrical (224) XRD confirmed the compressive strain $\varepsilon_{\parallel}$ of the $Ge_{0.9}Sn_{0.1}$, estimated at $\sim -0.8\%$, as shown in Fig. S11c.

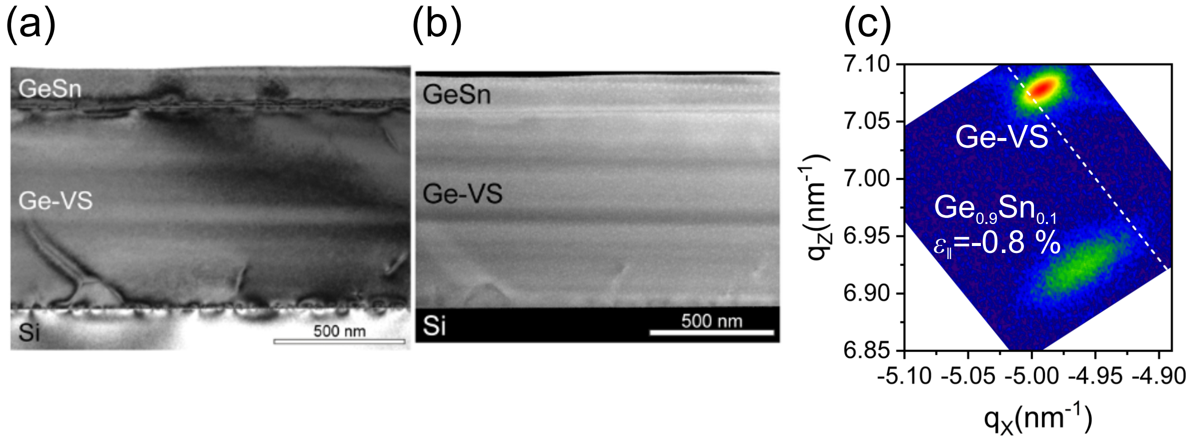


Figure S11. (a) Cross-sectional transmission electron microscopy (TEM) image of the $Ge_{0.9}Sn_{0.1}$ thin film grown on top of the 2 µm thick Ge-VS. The defects are mainly localized near the interfaces between Si/Ge and Ge/$Ge_{0.9}Sn_{0.1}$. Threading dislocation are contained within the Ge-VS. (b) Low magnification TEM image of the full stack. (c) Reciprocal space mapping (RSM) around the asymmetrical (224) XRD peak is performed for the reference $Ge_{0.9}Sn_{0.1}$ thin film to decouple the strain and composition in the layer. The compressive strain ($\varepsilon_{\parallel}$) was evaluated to be around -0.8%.

## Supplementary Note 9. Geometrical Parameters of the Core/Shell NW Array

The SEM measured geometrical parameters of the different Si/GeSn and Si/Ge core/shell NWs are presented in Table S4. All geometrical parameters are defined in Fig. 1b of the main text. The error bar originates from statistical analysis of many NW based on the acquired SEM images.

TABLE S4. Geometrical parameters of the core/shell NW array. All dimensions are in nm.

| | Si NW array | Si/Ge NWs | | | Si/GeSn NWs |
|---|---|---|---|---|---|
| $d_{cT}$ (nm) | $20 \pm 2$ | $20 \pm 2$ | $20 \pm 2$ | $20 \pm 2$ | $35 \pm 1$ |
| $d_{cB}$ (nm) | $120 \pm 1$ | $120 \pm 1$ | $120 \pm 1$ | $120 \pm 1$ | $145 \pm 1$ |
| $d_{sT}$ (nm) | N/A† | $40 \pm 6$ | $120 \pm 10$ | $180 \pm 10$ | $100 \pm 8$ |
| $d_{sB}$ (nm) | N/A | $160 \pm 9$ | $238 \pm 7$ | $288 \pm 12$ | $300 \pm 12$ |
| $a$ (nm) | N/A | N/A | N/A | N/A | $345 \pm 8$ |
| $b$ (nm) | N/A | N/A | N/A | N/A | $440 \pm 11$ |
| $u$ (nm) | | | $500 \pm 1$ | | |
| $h$ (nm) | N/A | N/A | N/A | N/A | $\sim 70 \pm 10$ |
| $H$ (nm) | N/A | $190 \pm 12$ | $207 \pm 10$ | $225 \pm 15$ | $354 \pm 10$ |
| $t$ (nm) | N/A | N/A | N/A | N/A | $128.5 \pm 5$ |

† N/A: Not Available

## References

[1] J. Q. Xi, M. F. Schubert, J. K. Kim, E. F. Schubert, M. Chen, S. Y. Lin, W. Liu, and J. A. Smart, Nat. Photonics **1**, 176 (2007).
[2] O. L. Muskens, J. G. Rivas, R. E. Algra, E. P. A. M. Bakkers, and A. Lagendijk, Nano Lett. **8**, 2638 (2008).
[3] T. Leontiou, J. Tersoff, and P. C. Kelires, Phys. Rev. Lett. **105**, 236104 (2010).
[4] J. Nicolas, S. Assali, S. Mukherjee, A. Lotnyk, and O. Moutanabbir, Cryst. Growth Des. **20**, 3493 (2020), 2003.01308.
[5] S. Assali, R. Bergamaschini, E. Scalise, M. A. Verheijen, M. Albani, A. Dijkstra, A. Li, S. Koelling, E. P. A. M. Bakkers, F. Montalenti, and L. Miglio, ACS Nano **14**, 2445 (2020).
[6] R. W. Olesinski and G. J. Abbaschian, Bulletin of Alloy Phase Diagrams **5**, 273 (1984).
[7] M. Albani, S. Assali, M. A. Verheijen, S. Koelling, R. Bergamaschini, F. Pezzoli, E. P. A. M. Bakkers, and L. Miglio, Nanoscale **10**, 7250 (2018).
[8] S. Assali, M. Albani, R. Bergamaschini, M. A. M. Verheijen, A. Li, S. Kölling, L. Gagliano, E. E. P. A. M. Bakkers, and L. Miglio, Applied Physics Letters **115**, 113102 (2019).
[9] Y. Yang, I. I. Kravchenko, D. P. Briggs, and J. Valentine, Nature Communications **5**, 5753 (2014).
[10] T. Ma, Q. Huang, H. He, Y. Zhao, X. Lin, and Y. Lu, Optics Express **27**, 16624 (2019).
[11] H. Yan, L. Huang, X. Xu, S. Chakravarty, N. Tang, H. Tian, and R. T. Chen, Optics Express **24**, 29724 (2016).
[12] S. Wang, Y. Liu, D. Zhao, H. Yang, W. Zhou, and Y. Sun, Applied Physics Letters **110**, 091105 (2017).
[13] W. He, W. Zhang, J. Zhang, P. Yu, P. Liu, G. Yang, and H. Lei, Applied Physics Letters **119**, 111106 (2021).
[14] R. Alaee, C. Rockstuhl, and I. Fernandez-Corbaton, Optics Communications **407**, 17 (2018).
[15] T. Hinamoto and M. Fujii, OSA Contin. **4**, 1640 (2021).
[16] M. Newville, T. Stensitzki, D. B. Allen, and A. Ingargiola, Lmfit: Non-linear least-square minimization and curve-fitting for python (2014).
